# Supplementary material for: State-Free Inference of State-Space Models: The Transfer Function Approach
Source: arXiv:2405.06147 source file (2024-06-02)
Supplement: Supplementary file 1 [file code.tex]

\newpage
\subsection{\texttt{PyTorch} Implementation} \label{app:code}

A simplified \texttt{PyTorch} \cite{pytorch} implementation of RTF is provided below.

\begin{lstlisting}[language=Python]
import torch
import torch.nn as nn
from torch.nn.functional import pad
from torch.fft import rfft, irfft
from einops import repeat, rearrange

class RTF(nn.Module):
    def __init__(self, state_size:int, channels:int, l_max:int):
        super().__init__()
        self.N, self.C, self.L = state_size, channels, l_max
        self.b_ = nn.Parameter(torch.zeros(self.N, self.C))
        self.a = nn.Parameter(torch.zeros(self.N, self.C))
        self.h_0 = nn.Parameter(torch.ones(self.C))
    
    @property
    def K_(self): # computes conv. kernel
        ba = torch.cat((self.b_, self.a), dim=1) # concat for parallel padding, and rfft
        ba = pad(ba, (0,0,1,self.L-self.N+self.L%2-1)) 
        ba[0,self.C:] = 1 # set monic term of denom
        BA = rfft(ba, dim=0)
        K = BA[:,:self.C]/BA[:,self.C:] + self.h_0
        return K

    def forward(self, u): # parallel inference
        L = u.size(-2)
        L_ = 2*L-L%2
        k_ = irfft(self.K_,dim=0)[:L] # below this point is the FFTConv, same as S4, S4D, etc.
        u = rearrange(u, "B L C -> L (B C)")
        KU = rfft(torch.cat((k_,u),dim=1),n=L_, dim=0)
        U = rearrange(KU[:,self.C:], "L (B C) -> B L C", C=self.C)
        Y = KU[:,:self.C]*U
        y = irfft(Y, dim=-2, n=L_)[:,:L]
        return y

    def step(self, u, x_i): # recurrent inference
        b, a, D = self.b, self.a.flip(dims=[0]), self.h_0 # self.b can be cached
        y = torch.einsum("BNC,NC->BC", x_i, b) + D*u
        x_f = torch.roll(x_i, -1, 1)
        x_f[:,-1] = torch.einsum("NC,BNC->BC",-a,x_i) + u
        return y, x_f

    @property
    @torch.no_grad()
    def b(self): # numerator correction
        dev = self.h_0.device
        A = torch.roll(torch.eye(self.N, device=dev),-1,0)
        A = torch.clone(repeat(A, "N M -> N M C",C=self.C))
        A[-1] = -self.a.flip(dims=[0])
        AL = torch.matrix_power(rearrange(A, "N M C -> C N M"), self.L)
        I_AL = torch.eye(self.N, device=dev) - AL
        return torch.linalg.solve(I_AL, self.b_.flip(dims=[0]).T, left=True).T

    def x_0(self, batch_shape, device=None): # default state
        return torch.zeros(batch_shape, self.N, self.C, device=device)
\end{lstlisting}
