# Supplementary material for: State-Free Inference of State-Space Models: The Transfer Function Approach
Source: arXiv:2405.06147 source file (2024-06-02)
Supplement: Supplementary file 2 [file proofs.tex]

\newpage
\section{Proofs}
